# Supplementary material for: ResFed: Communication Efficient Federated Learning by Transmitting Deep Compressed Residuals
Source: arXiv:2212.05602 source file (2022-12-11)
Supplement: Supplementary file 1 [file B_appendix.tex]

\section{Appendix B}
\label{sec:app_b}
\subsection{Preliminaries}

\begin{equation}
    \label{Eq:Video_codec}
    \hat{x}_t = f_{dec}(quantization (f_{enc}(x_t - \Tilde{x}_t))) + \Tilde{x}_t \text{~~~~} \text{where} \text{~~~~} \Tilde{x}_t = f_{pred}(\hat{x}_{t-1})
\end{equation}

\begin{equation}
    \label{Eq:client_pre}
    \hat{w}^t = f_{dec}(quantization (f_{enc}(w^t - \Tilde{w}^t))) + \Tilde{w}^t \text{~~~~} \text{where} \text{~~~~} \Tilde{w}^t = f_{pred}(\hat{w}^{t-1})
\end{equation}

\begin{equation}
    \label{Eq:client_pre}
    w^{t+1}_k = w^{t} + \eta \nabla F_k(w^{t}) \text{~~~~} \text{where} \text{~~~~} F_K(w^{t}) =  \frac{1}{n_k} \sum_{i=1}^{n_k} f_i(w^{t})
\end{equation}

\begin{equation}
    \label{Eq:server_pre}
    w^{t+1} = \frac{n_k}{n}\sum_k {w}_k^{t}
\end{equation}

compression for NUR uploading:

\begin{equation}
    \label{Eq:localupdate}
    w^{t+1} = \frac{n_k}{n}\sum_k \hat{w}_k^{t}
\end{equation}

compression for NUR downloading. Client runs SGD for only one epoch:

\begin{equation}
    \label{Eq:localupdate}
    w^{t+1}_k = w^{t} + \eta \nabla F_k(\hat{w}^{t}) \text{~~~~} \text{where} \text{~~~~} F_K(\hat{w}^{t}) =  \frac{1}{n_k} \sum_{i=1}^{n_k} f_i(\hat{w}^{t})
\end{equation}

%%%%%%%%%%%%%%%%%%%%%%%%%%%%%%%%%%%%%%%%%%%%%%%%
\begin{comment}

\begin{equation}
    \label{Eq:localupdate}
    \hat{w}^{t+1}_k = \hat{w}_t + \eta \nabla F_k(\hat{w}_t) \text{~~~~} \text{where} \text{~~~~} F_K(\hat{w}_t) =  \frac{1}{n_k} \sum_{i=1}^{n_k} f_i(\hat{w}_t)
\end{equation}

\begin{equation}
    \label{Eq:localupdate}
    \epsilon_i^t = f_i(\hat{w}_t) - f_i({w}_t)
\end{equation}

\begin{equation}
    \label{Eq:localupdate}
    \hat{w}^{t+1}_k = \hat{w}_t + \eta \nabla F_k(\hat{w}_t) \text{~~~~} \text{where} \text{~~~~} F_K(\hat{w}_t) =  \frac{1}{n_k} \sum_{i=1}^{n_k} (f_i({w}_t) + \epsilon_i^t)
\end{equation}

\begin{equation}
    \label{Eq:localupdate}
    \hat{w}^{t+1}_k = \hat{w}_t + \eta \nabla \frac{1}{n_k} \sum_{i=1}^{n_k} (f_i({w}_t) + \epsilon_i^t)
\end{equation}

\begin{equation}
    \label{Eq:localupdate}
    \hat{w}^{t+1}_k = \hat{w}_t + \eta \nabla F_k(\hat{w}_t) \text{~~~~} \text{where} \text{~~~~} F_K(\hat{w}_t) =  \frac{1}{n_k} \sum_{i=1}^{n_k} f_i(\hat{w}_t)
\end{equation}

\begin{equation}
    \label{Eq:globalupdate}
  w^{t+1}_k = w^{t} + \eta \nabla f(w) \text{~~~~} \text{where} \text{~~~~} f(w)=\sum_{k=1}^{K} \frac{n_k}{n} F_k(w)
\end{equation}

\begin{equation}
    \label{Eq:localupdate}
    w^{t+1}_k = w^{t} + \eta \nabla f(w)
\end{equation}

\end{comment}
