# Supplementary material for: ResFed: Communication Efficient Federated Learning by Transmitting Deep Compressed Residuals
Source: arXiv:2212.05602 source file (2022-12-11)
Supplement: Supplementary file 2 [file algorithm_sim.tex]

\begin{algorithm}[h]%Consider splitting the algo into server and client parts or use another template.
 \Reviewb{
 \caption{\raggedright: \Reviewb{Simplified residual-based federated learning framework}}
 \label{alg:FedRes}
 \begin{algorithmic}[1]

    \State \textbf{Server runs:} 
    \State initialize the global model, empty local and global model trajectories, and the predictor at the server
    \For{$i \in \{1,2,...,N\}$}
       \State initialize empty local and global model trajectories, and the predictor
       \State share the predictors
    \EndFor
    \For{each communication round}
        \For{each client \textbf{in parallel}}
            \If{$t < T$}
                \State do normal federated learning and update trajectories
            \Else
            \State \Reviewa{server communicates $\bar r_{i,dl}$ to the client $i$}
            \State $\bar r_{i,ul} \leftarrow$
            \textbf{ResFedClientUpdate} $(i, \bar r_{i,dl})$ \Comment{@client $i$}
            \State \Reviewa{client $i$ communicates $\bar r_{i,ul}$ to the server}
            \State recovery models $\hat w_i$ based on predicted models $\tilde w_i$
            \EndIf
         \State update local trajectory at the server
        \EndFor
        \State $w \leftarrow \textbf{Aggregate}(\hat w_1,...,\hat w_N)$
        \For {each client}
            \State compute residuals $r_{i,dl}$ based on predicted model $\tilde w_i$
            \State compress residuals $\bar r_{i,dl}$ and synchronize global trajectory
        \EndFor
    \EndFor
    \State \textbf{return} $w$ 
    \vspace{0.2cm}
    \State \textbf{ResFedClientUpdate} $(k, \bar r)$
    \State recover models $\hat w$ based on predicted models
    \State update global trajectory
    \State $w_k \leftarrow \textbf{LocalTrain}(\hat w)$
    \State compute residuals $r_k$ based on predicted models $\tilde w$
    \State compress residuals $\bar r_k$ and synchronize global trajectory
    \State \textbf{return} $\bar r_k$

\end{algorithmic}}
\end{algorithm}
