# Supplementary material for: ResFed: Communication Efficient Federated Learning by Transmitting Deep Compressed Residuals
Source: arXiv:2212.05602 source file (2022-12-11)
Supplement: Supplementary file 3 [file A_appendix.tex]

\section{Detail Information of used Federated Datasets}
\label{sec:app_a}

In the federated learning problem, we are given a set of clients indexed by $k$, in each a machine learning model with weights $w_k$ is trained on local datasets, $\{(x_i, y_i)|i=1,2,...,n_k\}$, where $(x_i, y_i)$ is one data point with label in client $k$, the number of the local data points is $n_k$. The local dataset is also notated as $(X_k, y_k)$, where $X_k \in \mathbb{R}^{n_k\times d}$ and $y_k \in \mathbb{R}^{n_k\times C_k}$, $C_k$ is then the number of classes in the local dataset. As we consider the datasets across clients can be Non-IID, the distribution of the datasets in client $k$ is notated as $D_k$, i.e. $(x_i, y_i)\in D_k$. 

Guided by federated learning benchmark datasets in~\cite{https://doi.org/10.48550/arxiv.1812.01097}, we assign each client only two classes, i.e. $\forall{k \in \{1,2,...,K\}}: C_k = 2$. As the unbalance issue with is addressed in \emph{FedAvg}~\cite{pmlr-v54-mcmahan17a}, we provide balanced partition of the data in our experiment, i.e. given two indices of client $p$ and $q$, $\{p, q\}\supset \{1,2,...,K\}$, then $n_p \approx n_q$.

\noindent\textbf{MNIST}

\noindent\textbf{IMAGENET}
