# Supplementary material for: ResFed: Communication Efficient Federated Learning by Transmitting Deep Compressed Residuals
Source: arXiv:2212.05602 source file (2022-12-11)
Supplement: Supplementary file 4 [file A_effectiveness.tex]

Convergence

Assume the function is a Local Lipschitz continuity of the function $f$
\begin{equation}
    ||\nabla f(\hat w) - \nabla f(w_i)|| \leq L||\hat w - w_i||
\end{equation}

Based on the L-Lipschitz smoothness of f and Taylor expansion
\begin{equation}
    f(w_i) = f(\hat w + (w_i -\hat w)) \leq f(\hat w) + \nabla f(\hat w)^T(w_i -\hat w)+\frac{1}{2}L||w_i - \hat w||^2_2
\end{equation}

\begin{equation}
    \leq f(\hat w) - (1 - \frac{1}{2}L\eta)\eta||\nabla f(\hat w)||^2_2
\end{equation}

\begin{equation}
    f(w_i^t)-f(w_i^*)\leq \frac{||w_i^t-w_i^*||^2_2}{2\eta t} 
\end{equation}

\begin{equation}
    r_i^{t+1} \leq (\frac{t-1}{4\eta t(t+1) })||w_i^t-w_i^*||^2_2 \leq w_i^{t+1}
\end{equation}
