# Supplementary material for: ResFed: Communication Efficient Federated Learning by Transmitting Deep Compressed Residuals
Source: arXiv:2212.05602 source file (2022-12-11)
Supplement: Supplementary file 5 [file extended_discussion.tex]

\section{Extended Discussion}

In Sec.\ref{sec:warmup}, we discuss the potential enhancement from warn-up communication rounds, which has been employed in the previous work~\cite{lin2018deep} to increase the compression ratio for deep gradient compression.\Rui{tbd.}

Additionally, we provide primary evaluation on security improvement from \myResFed in Fig.~\ref{}\Rui{tbd.}, which is discussed in Sec.~\ref{sec:security}.
